# Supplementary material for: Deep-Learning-Based Precipitation Nowcasting with Ground Weather Station Data and Radar Data
Source: arXiv:2210.12853 source file (2022-10-20)
Supplement: Supplementary file 1 [file 099appendix.tex]

\begin{table}[t]
    \centering
    \caption{CSI scores of predicting \textsc{Heavy} and \textsc{Heavy+Light} on test set}
    \setlength{\tabcolsep}{4pt}
    \begin{tabular}{c|c|cc|cc|cc}
        \toprule
        \multirow{2}{*}{\makecell{Precipitation \\ level}} & \multirow{2}{*}{Lead time} & \multicolumn{2}{c|}{\method} & \multicolumn{2}{c|}{LSTM} & \multicolumn{2}{c}{Persistence} \\
        & & CSI & F1 & CSI & F1 & CSI & F1 \\
        \midrule
        \multirow{7}{*}{\makecell{\textsc{Heavy} \\ ($\geq$10mm/h)}} & $60$ minutes & 0.291 & 0.451 & 0.296 & 0.457 & 0.259 & 0.412\\
        & $120$ minutes & 0.197 & 0.329 & 0.178 & 0.302 & 0.152 & 0.264\\
        & $180$ minutes & 0.147 & 0.257 & 0.127 & 0.225 & 0.102 & 0.185\\
        & $240$ minutes & 0.111 & 0.199 & 0.090 & 0.166 & 0.073 & 0.136\\
        & $300$ minutes & 0.082 & 0.151 & 0.064 & 0.121 & 0.057 & 0.108\\
        & $360$ minutes & 0.062 & 0.117 & 0.048 & 0.091 & 0.046 & 0.087\\
        \cmidrule{2-8}
        & Average & 0.148 & 0.251 & 0.134 & 0.227 & 0.115 & 0.199 \\
        \midrule\midrule
        \multirow{7}{*}{\makecell{\textsc{Heavy+} \\ \textsc{Light} \\ ($\geq$1mm/h)}} & $60$ minutes & 0.525 & 0.689 & 0.527 & 0.690 & 0.518 & 0.683 \\
        & $120$ minutes & 0.423 & 0.594 & 0.408 & 0.580 & 0.396 & 0.568 \\
        & $180$ minutes & 0.366 & 0.535 & 0.347 & 0.515 & 0.331 & 0.498 \\
        & $240$ minutes & 0.322 & 0.488 & 0.306 & 0.468 & 0.288 & 0.447 \\
        & $300$ minutes & 0.288 & 0.448 & 0.275 & 0.432 & 0.256 & 0.408 \\
        & $360$ minutes & 0.260 & 0.413 & 0.250 & 0.401 & 0.231 & 0.375 \\
        \cmidrule{2-8}
        & Average & 0.364 & 0.528 & 0.352 & 0.514 & 0.337 & 0.496 \\
        \bottomrule
    \end{tabular}
    \label{tab:q1_result_aws}
\end{table}

\begin{table*}[t]
    \centering
    \caption{CSI scores of predicting \textsc{Heavy} and \textsc{Heavy+Light} on test set}
    \begin{tabular}{c|c|cc|C{1cm}C{1cm}|C{1cm}C{1cm}|C{0.75cm}C{0.75cm}}
        \toprule
        \multirow{2}{*}{\makecell{Precipitation \\ level}} & \multirow{2}{*}{Lead time} & \multicolumn{2}{c|}{\adv} & \multicolumn{2}{c|}{DeepRaNE + kriging} & \multicolumn{2}{c|}{DeepRaNE + LSTM} & \multicolumn{2}{c}{DeepRaNE only} \\
        & & CSI & F1 & CSI & F1 & CSI & F1 & CSI & F1 \\
        \midrule
        \multirow{6}{*}{\makecell{\textsc{Heavy} \\ ($\geq$10mm/h)}} & $60$ minutes & 0.444 & 0.615 & 0.316 & 0.480 & \textbf{0.464} & \textbf{0.634} & 0.390 & 0.562 \\
        & $120$ minutes & \textbf{0.309} & \textbf{0.472} & 0.200 & 0.333 & 0.285 & 0.443 & 0.280 & 0.438 \\
        & $180$ minutes & \textbf{0.218} & 0.357 & 0.158 & 0.273 & \textbf{0.218} & \textbf{0.358} & 0.210 & 0.348 \\
        & $240$ minutes & 0.169 & 0.289 & 0.128 & 0.226 & 0.154 & 0.267 & \textbf{0.170} & \textbf{0.291} \\
        & $300$ minutes & \textbf{0.141} & \textbf{0.247} & 0.108 & 0.195 & 0.125 & 0.222 & 0.135 & 0.238 \\
        & $360$ minutes & 0.096 & 0.176 & 0.092 & 0.168 & 0.094 & 0.172 & \textbf{0.116} & \textbf{0.207} \\
        \midrule\midrule
        \multirow{6}{*}{\makecell{\textsc{Heavy+} \\ \textsc{Light} \\ ($\geq$1mm/h)}} & $60$ minutes & \textbf{0.671} & \textbf{0.803} & 0.483 & 0.652 & 0.670 & 0.802 & 0.609 & 0.757 \\
        & $120$ minutes & 0.548 & 0.708 & 0.409 & 0.581 & \textbf{0.550} & \textbf{0.710} & 0.501 & 0.667 \\
        & $180$ minutes & 0.468 & 0.638 & 0.375 & 0.546 & \textbf{0.477} & \textbf{0.646} & 0.449 & 0.620 \\
        & $240$ minutes & \textbf{0.428} & \textbf{0.599} & 0.339 & 0.507 & 0.425 & 0.596 & 0.411 & 0.583 \\
        & $300$ minutes & \textbf{0.394} & \textbf{0.565} & 0.315 & 0.479 & 0.390 & 0.561 & 0.381 & 0.552 \\
        & $360$ minutes & 0.359 & 0.529 & 0.294 & 0.454 & \textbf{0.365} & \textbf{0.535} & 0.354 & 0.523 \\
        \midrule\midrule
        \multicolumn{2}{c|}{Average} & \textbf{0.353} & \textbf{0.499} & 0.268 & 0.408 & 0.351 & 0.496 & 0.334 & 0.482 \\
        \bottomrule
    \end{tabular}
    \label{tab:q1_result}
\end{table*}
